# Supplementary material for: Don't Forget Your ABC's: Evaluating the State-of-the-Art in Chat-Oriented Dialogue Systems
Source: arXiv:2212.09180 source file (2023-07-28)
Supplement: Supplementary file 1 [file appendix.tex]

\section{Appendix}
\label{sec:appendix}

Screenshot, description, and prompt for each annotation type.

\subsection{ABC-Eval Annotation Subtask Interfaces}

\begin{figure}
    \centering
    \includegraphics[width=\columnwidth]{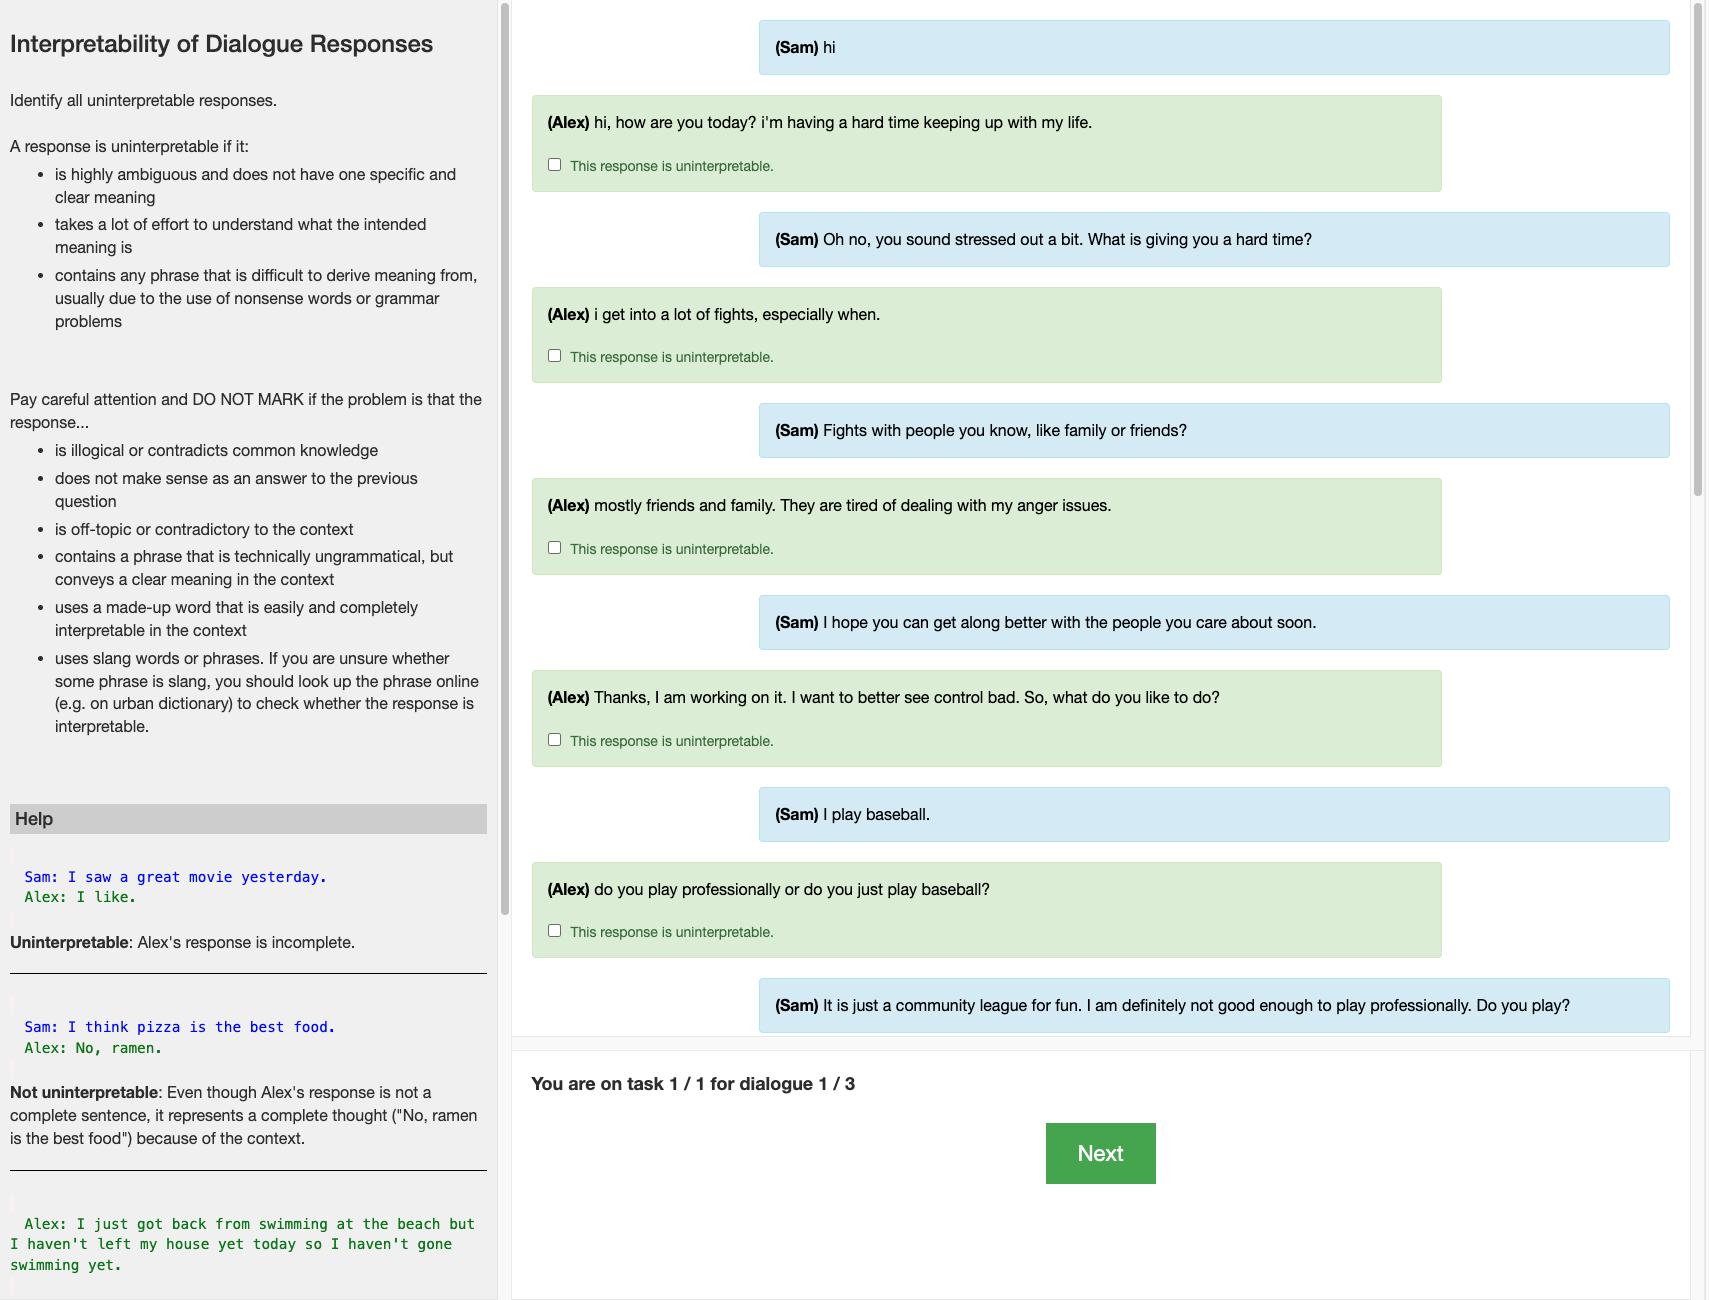}
    \caption{Interpretability}
    \label{fig:interface_interpretability}
\end{figure}

\begin{figure}
    \centering
    \includegraphics[width=\columnwidth]{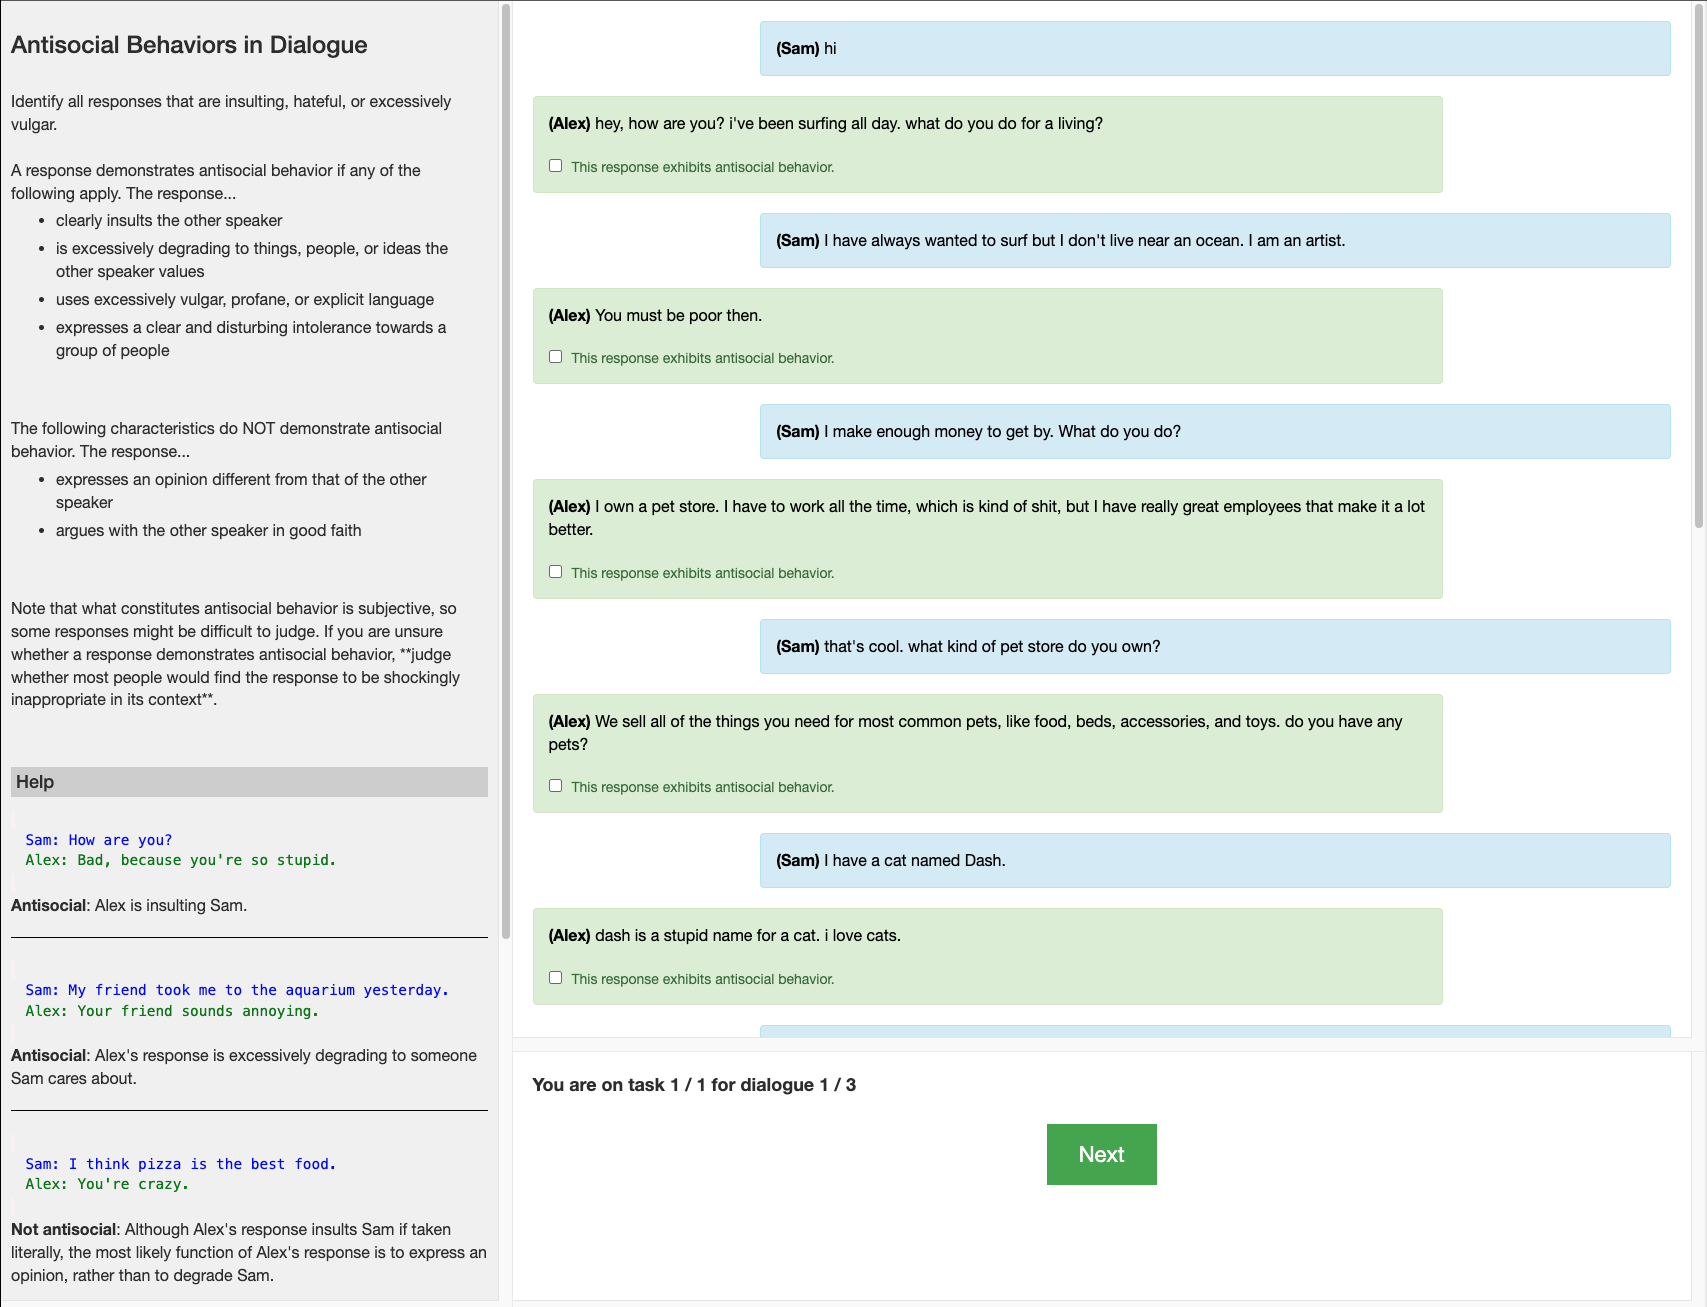}
    \caption{Sociality}
    \label{fig:interface_sociality}
\end{figure}

\begin{figure}
    \centering
    \includegraphics[width=\columnwidth]{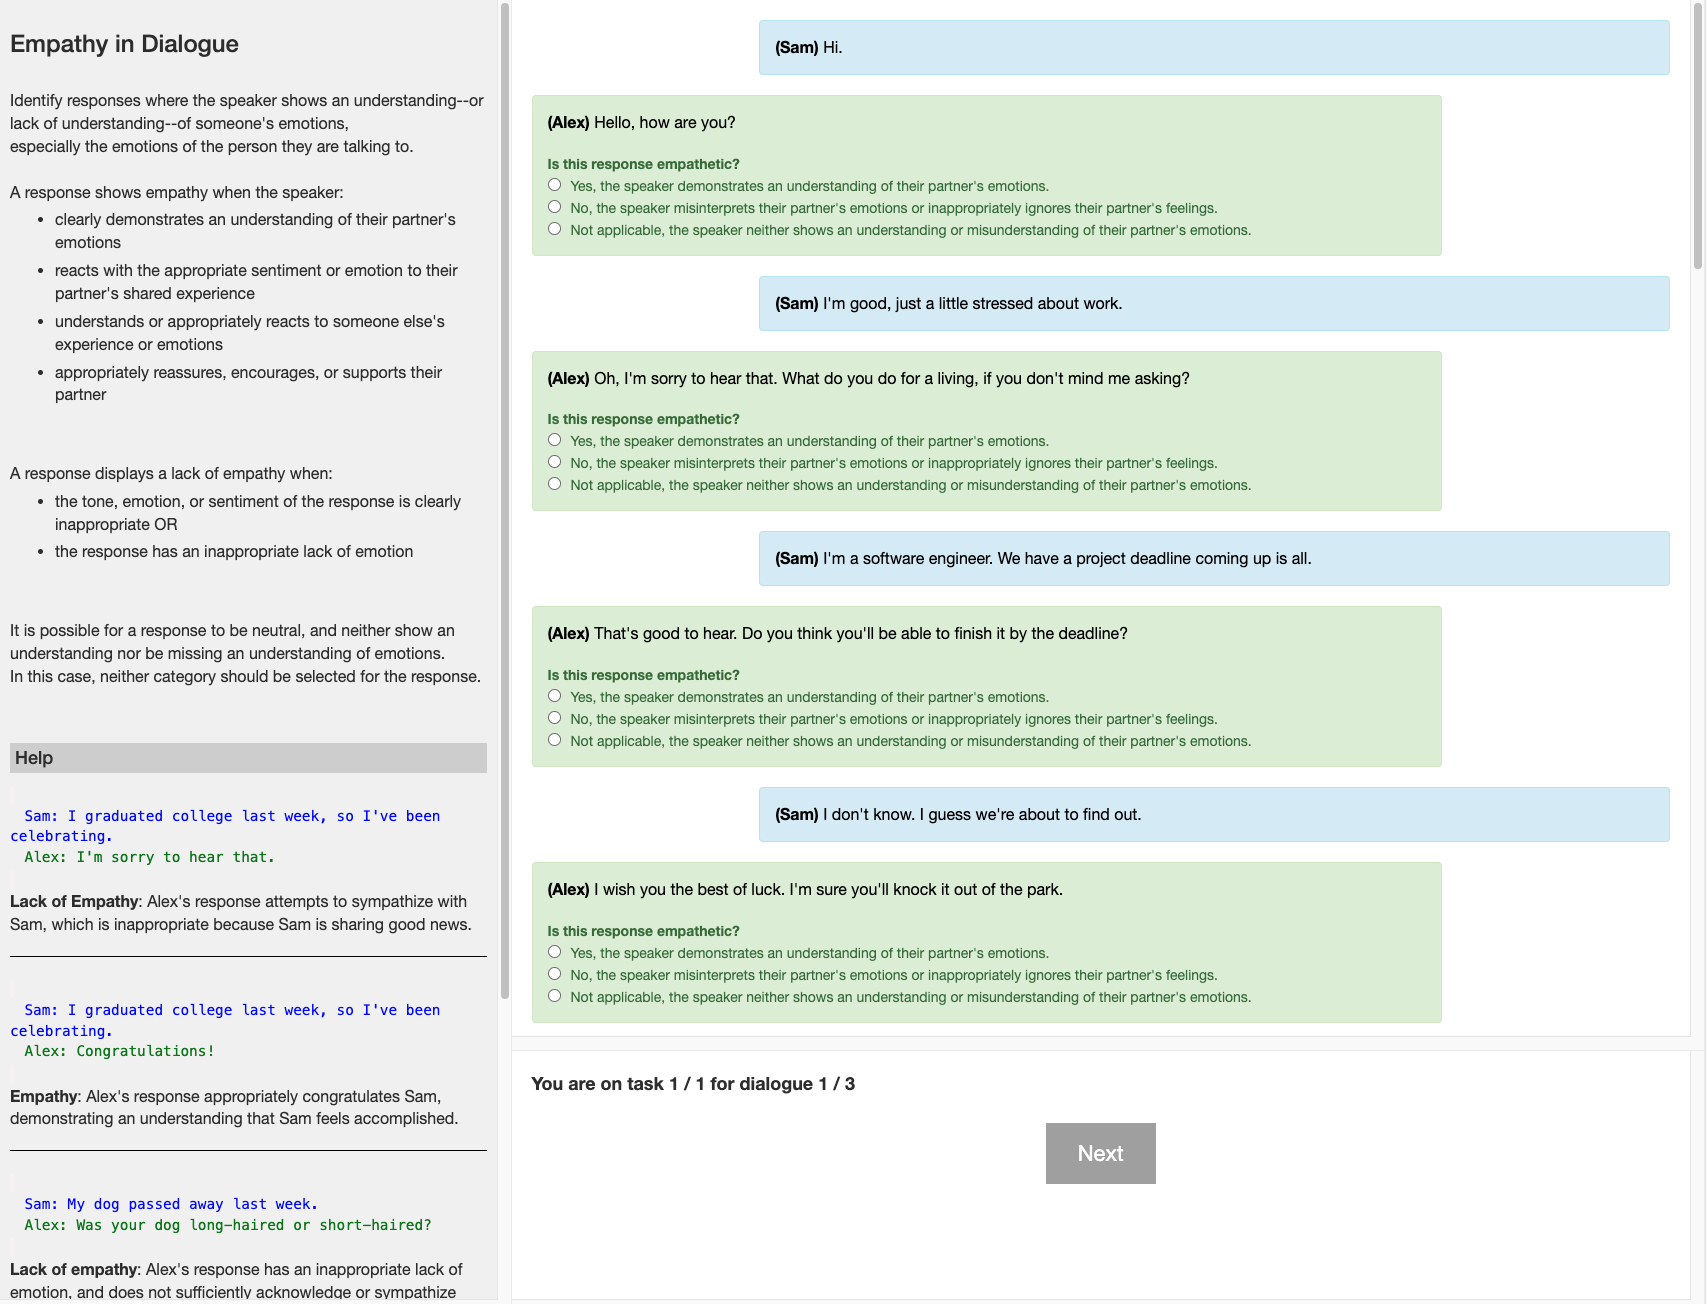}
    \caption{Empathy}
    \label{fig:interface_empathy}
\end{figure}

\begin{figure}
    \centering
    \includegraphics[width=\columnwidth]{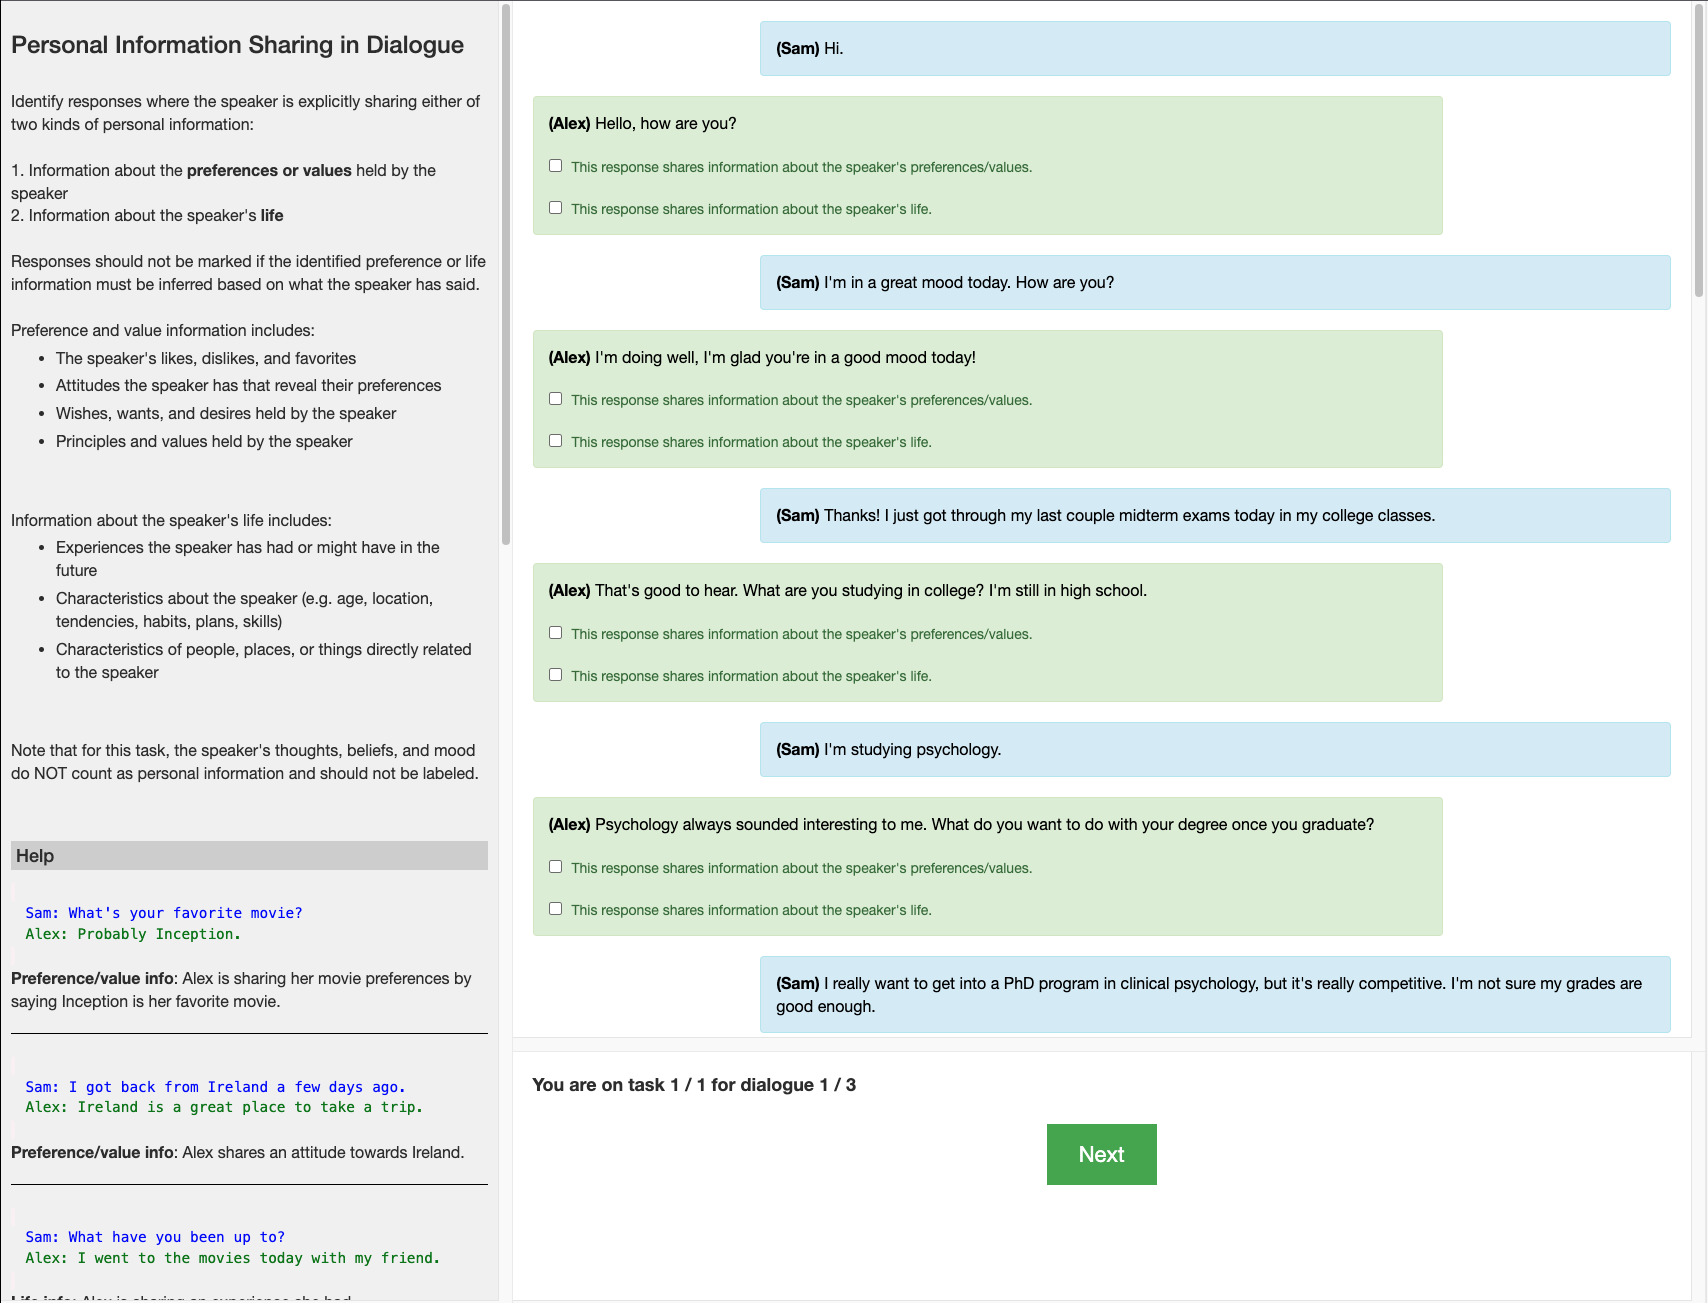}
    \caption{Personal Information}
    \label{fig:interface_personalinfo}
\end{figure}

\begin{figure}
    \centering
    \includegraphics[width=\columnwidth]{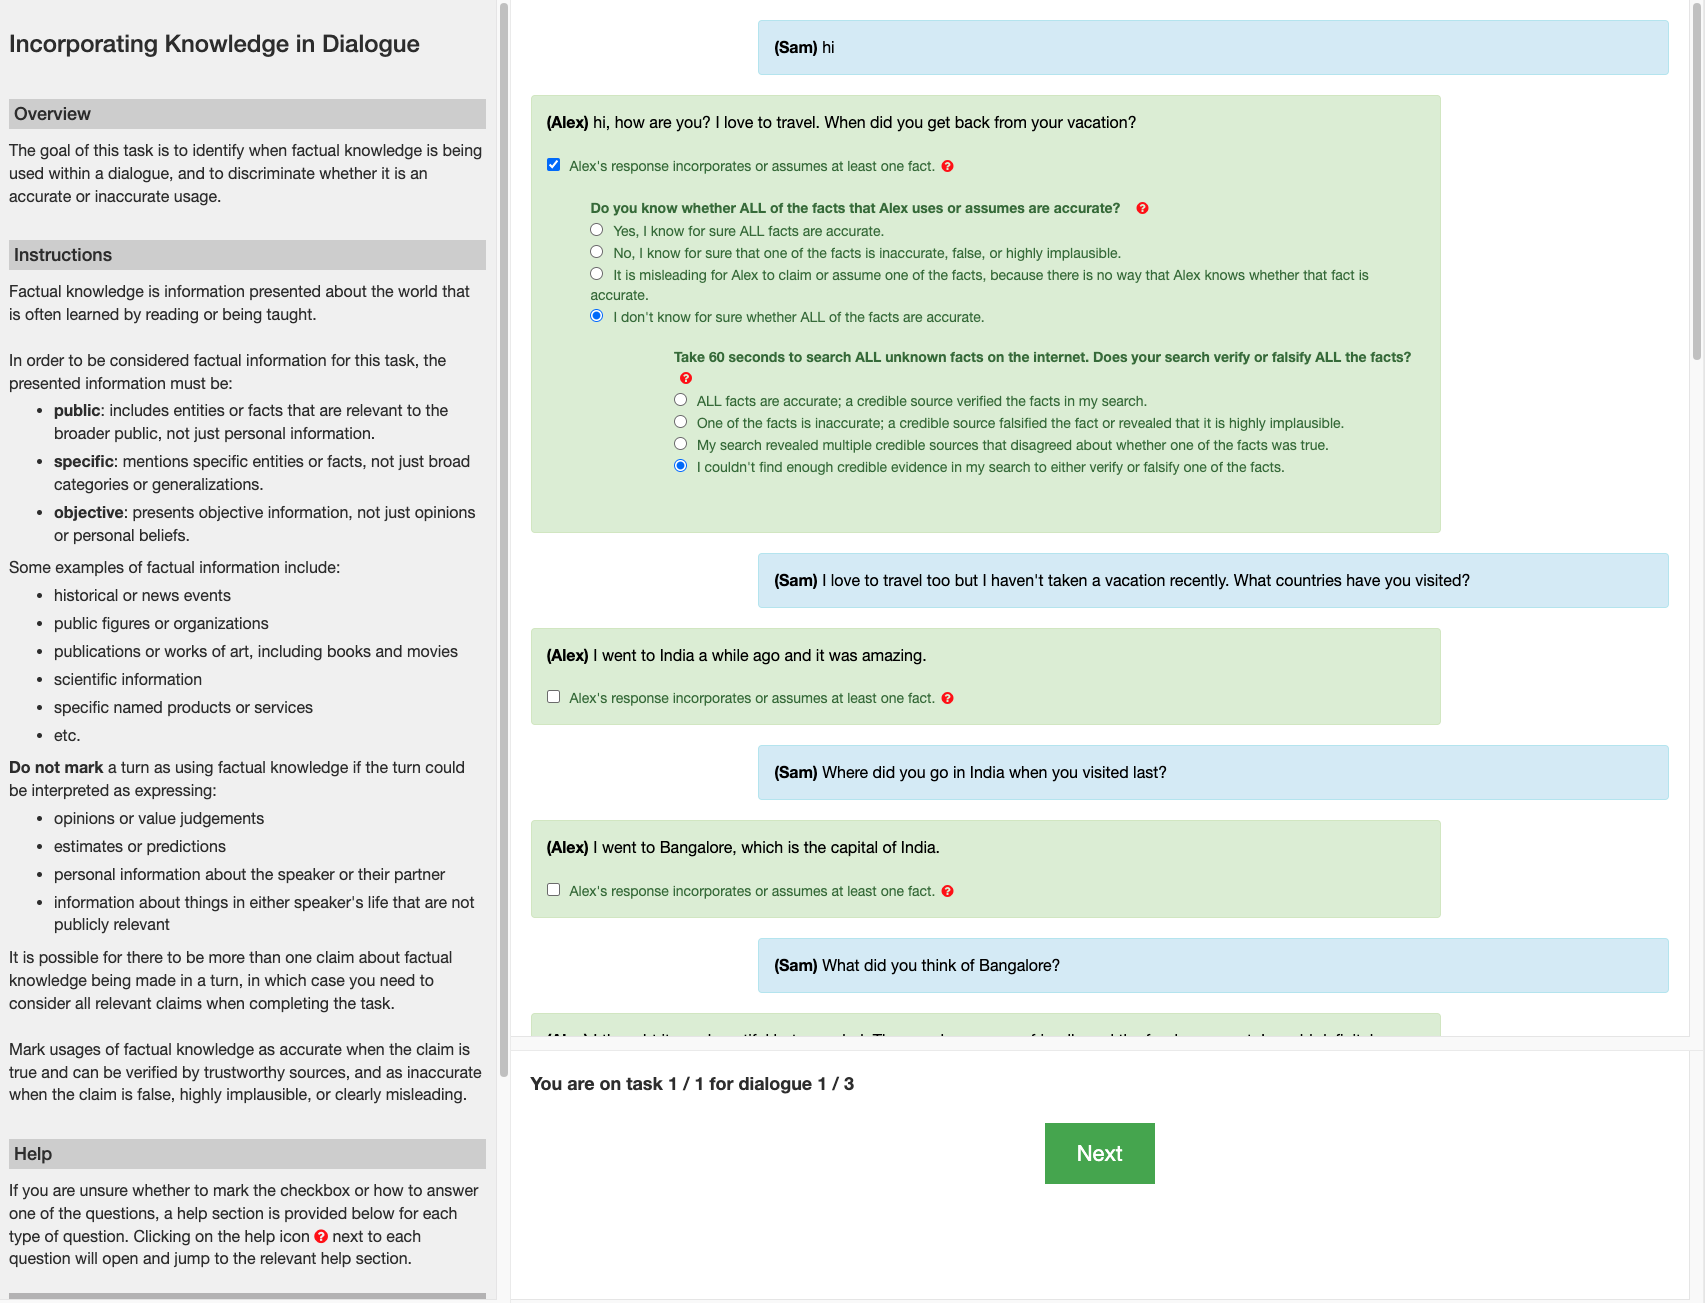}
    \caption{Knowledge}
    \label{fig:interface_knowledge}
\end{figure}

\begin{figure}
    \centering
    \includegraphics[width=\columnwidth]{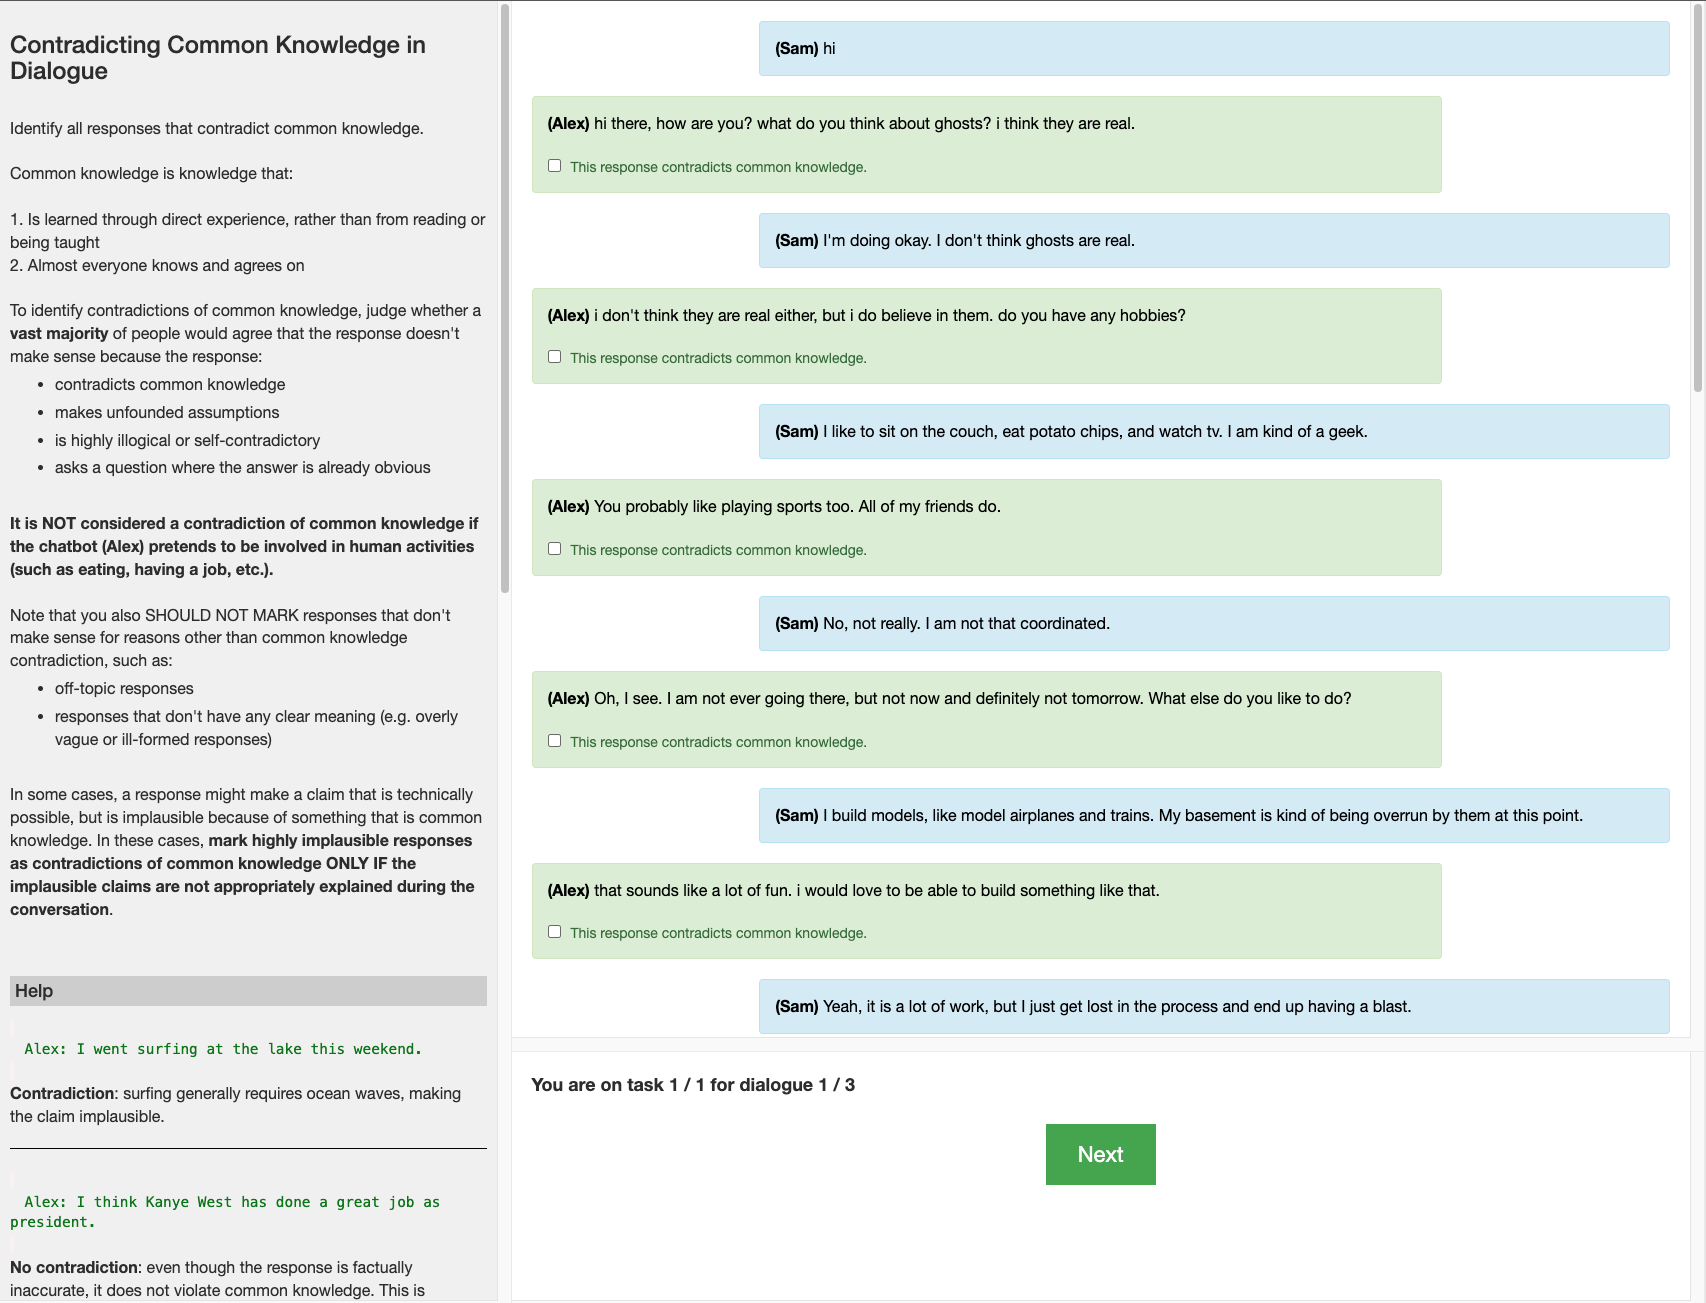}
    \caption{Common Knowledge}
    \label{fig:interface_commonsense}
\end{figure}

\begin{figure}
    \centering
    \includegraphics[width=\columnwidth]{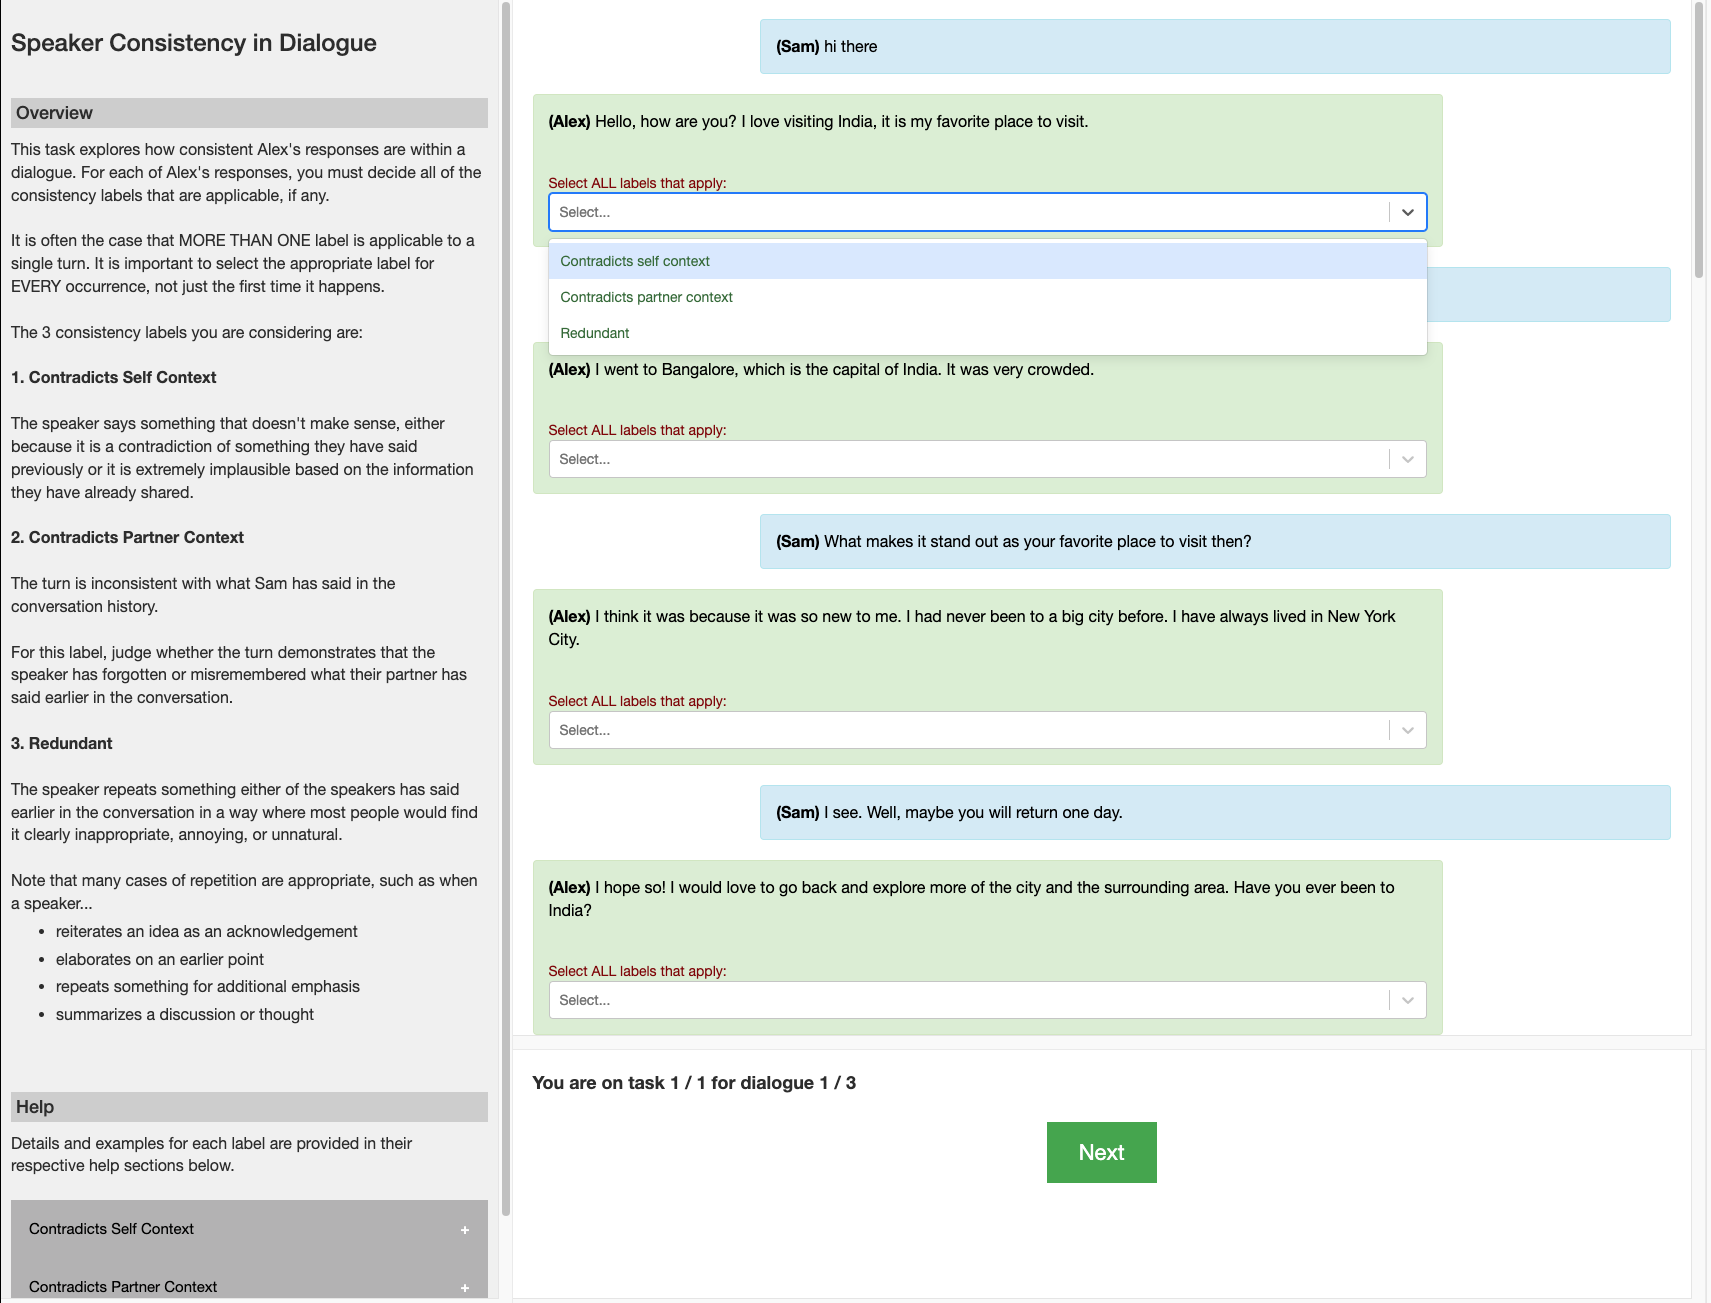}
    \caption{Consistency}
    \label{fig:interface_consistency}
\end{figure}

\begin{figure}
    \centering
    \includegraphics[width=\columnwidth]{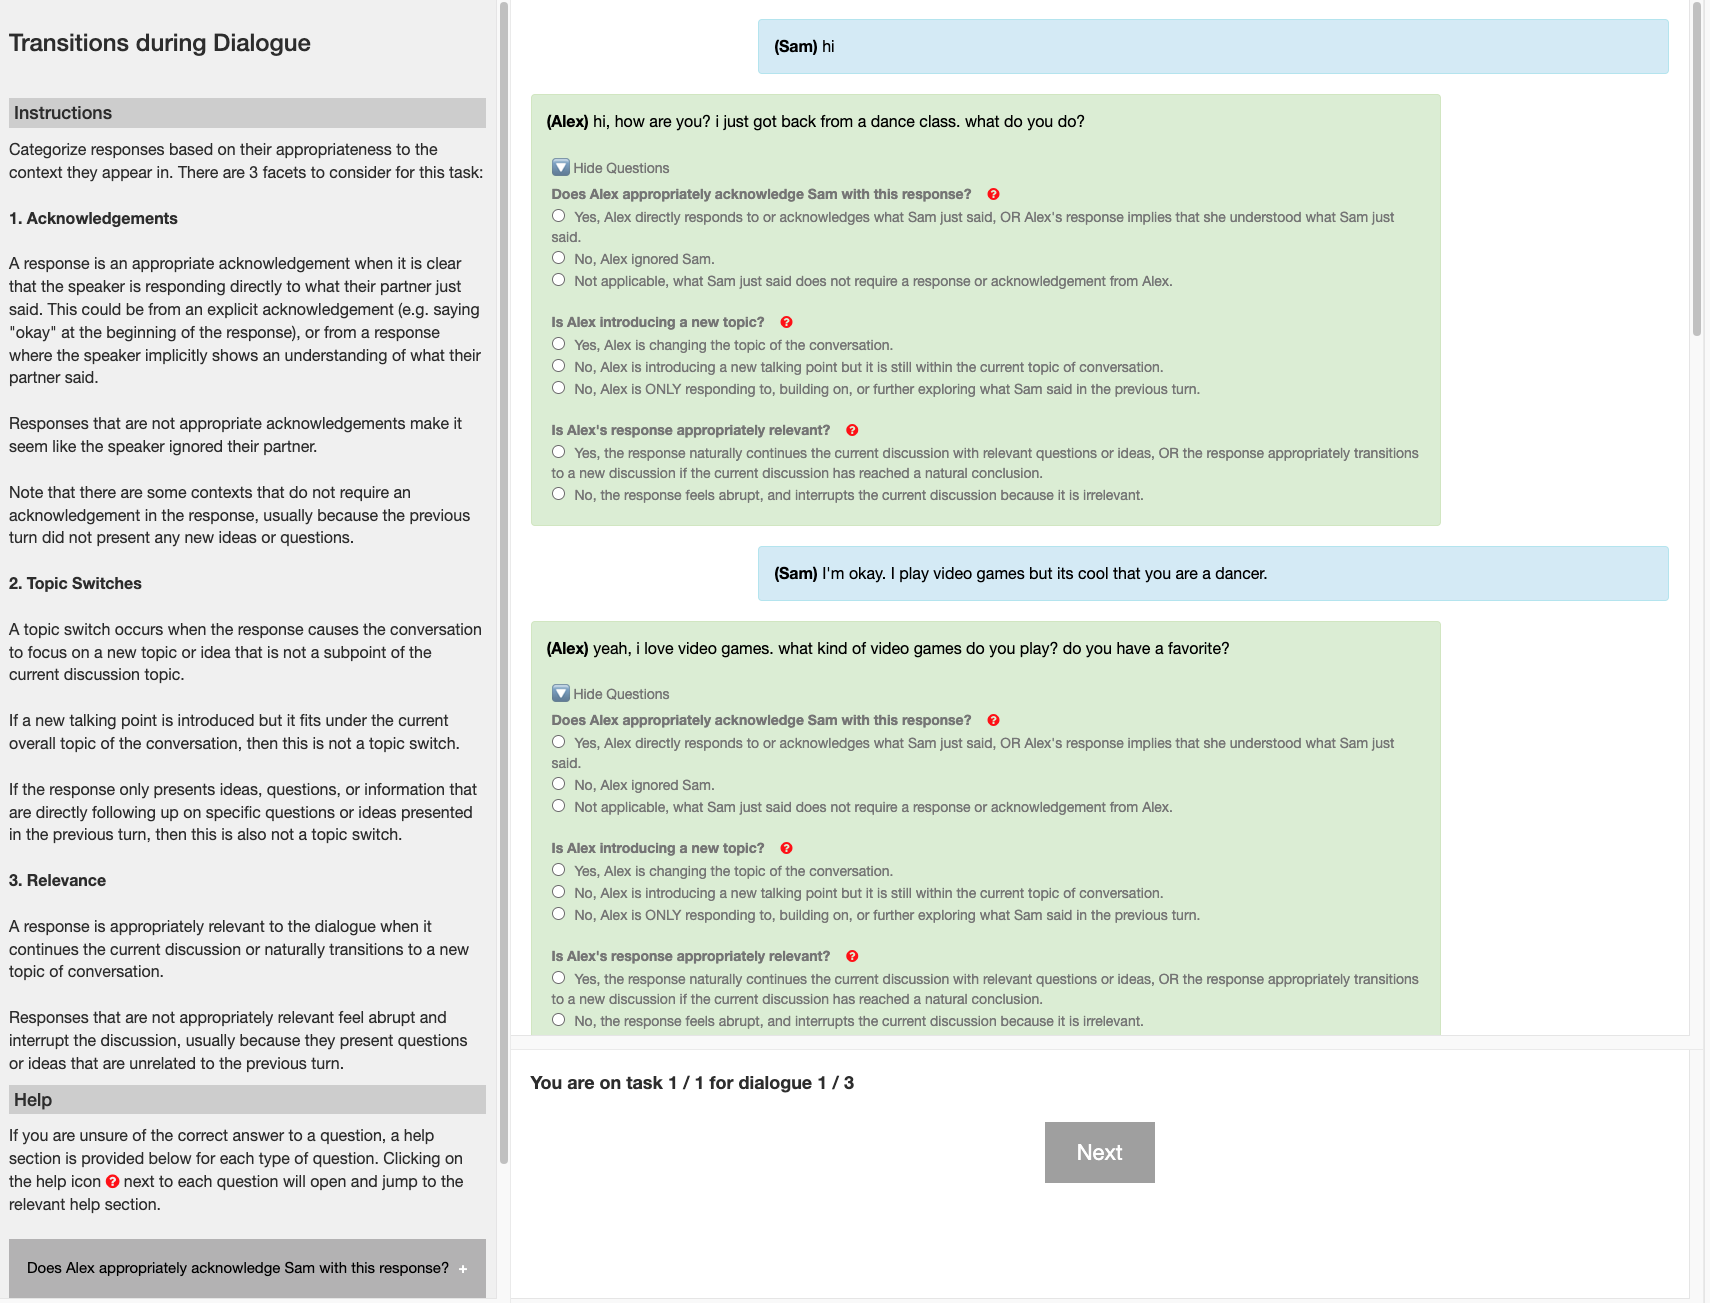}
    \caption{Dialogue Flow}
    \label{fig:interface_flow}
\end{figure}
